# Supplementary material for: Animating Childlike Drawings with 2.5D Character Rigs
Source: arXiv:2502.17866 source file (2025-02-25)
Supplement: Supplementary file 1 [file Appendix_A.tex]

\section{Annotation Study}

\subsubsection{Methodology}
399 images were selected from the Amateur Drawings Dataset~\cite{10.1145/3592788}, a crowd-sourced collection of childlike images. 199 images were randomly selected, but filtered by the research team to ensure that at least one figure body part suggested a side-facing orientation; the remaining 200 images were randomly selected without filtering.

A remote team of 15 professional annotators was contracted to provide annotations.
Using a browser-based interface, annotators observed each figure and determined whether the character appeared to be oriented more towards \textit{drawing left}, \textit{drawing right}, or, \textit{directly out of drawing.} 
If the orientation was towards \textit{drawing left} or \textit{drawing right}, they provided a free response identifying body parts and part traits that were used to infer orientation.
Because twisted perspective can result in different parts of a figure having different forward orientations, annotators did this independently for three different segments of the figure: head/face, upper trunk/arms, and lower trunk/legs.
Importantly, annotators were told that this was a subjective task with no correct answer.
Each figure was annotated by 10 different annotators.
Afterwards, a member of the research team randomly selected 3 annotations per image and coded the body parts and part traits mentioned in the free responses.

\subsubsection{Results}
\begin{table}[ht]
\small % Adjust font size
\centering
\begin{tabular}{|c|c|c|c|c|c|}
\hline
Figure Segment & Left & Right & Forward & Agreement & $\kappa$ \\
\hline
Head/Face & 1134 & 1068 & 1788 & 77\% & 0.65 \\
\hline
UpperTrunk/Arms & 130 & 316 & 3544 & 90\% & 0.50 \\
\hline
LowerTrunk/Legs & 616 & 856 & 2518 & 91\% & 0.83 \\
\hline
\end{tabular}
\caption{
Counts of how annotators labeled figure body part orientation.
We also calculate the percentage of the time observers agreed, along with Fleiss's kappa to account for by-chance agreement.
}
\label{table:annotation_orientation_frequency}
\end{table}

See Table~\ref{table:annotation_orientation_frequency} for the summary statistics about frequency and agreement between annotator labels.
Figure~\ref{fig:part_count_orientation} contains statistics about how frequently annotators mentioned specific body parts, as well as part trait, for the coded annotations.
Table~\ref{table:twisted_perpspective_frequency} contains statistics about how frequently figure were drawn with different segments oriented differently, as can be caused by twisting perspective. For this analysis, we use the most frequently chosen orientation as the `true' orientation of each figure's segment.
